# Supplementary material for: Improving compute efficacy frontiers with SliceOut
Source: arXiv:2007.10909 source file (2021-03-31)
Supplement: Supplementary file 1 [file Appendix_FashionMNIST_plots.tex]

\pgfplotsset{width=6.5cm,compat=1.9}
\begin{tikzpicture}
\begin{axis}[
    title={Cached GPU memory (\% of standard)},
    xlabel={Dropout rate},
    xmin=0, xmax=0.5,
    ymin=50, ymax=160,
    xtick={0,0.1,0.2,0.3,0.4,0.5},
    ytick={50,70,90,110,130,150},
    legend pos=south west,
    ymajorgrids=true,
    grid style=dashed,
    title style={font=\small},
    label style={font=\small},
    xtick label style={font=\small},
    ytick label style={font=\tiny},
    legend style={font=\tiny},
]
\addplot[color=red,mark=square,]
    coordinates {
    (0,100)(0.1,100)(0.2,100)(0.3,100)(0.4,100)(0.5,100)
    };
\addplot[color=blue,mark=o,]
    coordinates {
    (0,100)(0.1,93.2)(0.2,87)(0.3,81.5)(0.4,76.6)(0.5,73)
    };
\addplot[color=black,mark=+,]
    coordinates {
    (0,100)	(0.1,153.6)	(0.2,145.8)	(0.3,138.8)	(0.4,132.7)	(0.5,125.9)
    };
\legend{Standard, SliceOut, Controlled}
\end{axis}
\end{tikzpicture}
\hskip 0.5pt
\begin{tikzpicture}
\begin{axis}[
    title={Train time per epoch (\% of standard)},
    xlabel={Dropout rate},
    xmin=0, xmax=0.5,
    ymin=50, ymax=150,
    xtick={0,0.1,0.2,0.3,0.4,0.5},
    ytick={50,70,90,110,130,150},
    legend pos=south west,
    ymajorgrids=true,
    grid style=dashed,
    title style={font=\small},
    label style={font=\tiny},
    ytick label style={font=\tiny},
    legend style={font=\tiny},
]
\addplot[color=red,mark=square,]
    coordinates {
    (0,100)(0.1,100)(0.2,100)(0.3,100)(0.4,100)(0.5,100)
    };
\addplot[color=blue,mark=o,]
    coordinates {
    (0,100)(0.1,98.9)(0.2,95.3)(0.3,93.4)(0.4,90.5)(0.5,87.3)
    };
\addplot[color=black,mark=+,]
    coordinates {
    (0,100)	(0.1,148.3)	(0.2,132.1)	(0.3,116.4)	(0.4,103.7)	(0.5,92.3)
    };
\end{axis}
\end{tikzpicture}

\begin{tikzpicture}
\begin{axis}[
    title={Test accuracy Vs No. of epochs},
    xlabel={No. of epochs},
    xmin=0, xmax=100,
    ymin=60, ymax=100,
    xtick={0,20,40,60,80,100},
    ytick={60,70,80,90,100},
    legend pos=south west,
    ymajorgrids=true,
    grid style=dashed,
    title style={font=\small},
    label style={font=\small},
    xtick label style={font=\small},
    ytick label style={font=\tiny},
    legend style={font=\tiny},
]
\addplot[color=black,]
    coordinates {
    (1,79.17)	(2,82.41)	(3,83.86)	(4,84.74)	(5,84.71)	(6,85.63)	(7,85.96)	(8,86.2)	(9,86.38)	(10,86.43)	(11,86.6)	(12,86.85)	(13,86.75)	(14,87.34)	(15,87.14)	(16,87.5)	(17,87.11)	(18,87.23)	(19,87.75)	(20,87.91)	(21,88)	(22,87.8)	(23,87.89)	(24,88.06)	(25,88.26)	(26,88.34)	(27,88.48)	(28,88.06)	(29,88.45)	(30,88.12)	(31,88.41)	(32,87.62)	(33,88.39)	(34,88.4)	(35,88.42)	(36,88.68)	(37,88.78)	(38,88.59)	(39,88.44)	(40,88.78)	(41,88.7)	(42,88.71)	(43,88.55)	(44,88.79)	(45,88.66)	(46,88.7)	(47,88.76)	(48,88.74)	(49,88.63)	(50,88.74)	(51,88.57)	(52,88.67)	(53,88.6)	(54,88.75)	(55,88.64)	(56,89.09)	(57,89.1)	(58,89.12)	(59,88.86)	(60,88.99)	(61,88.98)	(62,89.07)	(63,88.9)	(64,88.92)	(65,89.05)	(66,88.81)	(67,88.99)	(68,88.88)	(69,88.93)	(70,89.13)	(71,89.18)	(72,89.11)	(73,89.05)	(74,88.85)	(75,89.19)	(76,89.19)	(77,88.97)	(78,88.93)	(79,89.08)	(80,89.16)	(81,88.85)	(82,89.16)	(83,89.39)	(84,89.12)	(85,89.17)	(86,89.33)	(87,89.18)	(88,89.21)	(89,89.18)	(90,89.29)	(91,89.25)	(92,88.88)	(93,89.16)	(94,89.05)	(95,89.17)	(96,89.34)	(97,89.07)	(98,89.3)	(99,89.31)	(100,89.32)
    };
\addplot[color=red,]
    coordinates {
    (1,78.57)	(2,81.81)	(3,83.71)	(4,84.39)	(5,84.76)	(6,85.21)	(7,85.29)	(8,85.62)	(9,85.98)	(10,86.26)	(11,86.42)	(12,86.7)	(13,86.68)	(14,87.04)	(15,87.27)	(16,87.28)	(17,87.19)	(18,87.26)	(19,87.48)	(20,87.43)	(21,87.64)	(22,87.48)	(23,87.75)	(24,87.82)	(25,87.84)	(26,87.74)	(27,87.85)	(28,87.83)	(29,87.95)	(30,88.06)	(31,88.08)	(32,88.05)	(33,87.82)	(34,87.99)	(35,88.12)	(36,88.14)	(37,87.95)	(38,88.04)	(39,88.34)	(40,88.04)	(41,88.11)	(42,88.23)	(43,88.18)	(44,88.32)	(45,88.14)	(46,88.35)	(47,88.23)	(48,88.29)	(49,88.09)	(50,88.31)	(51,88.31)	(52,88.33)	(53,88.35)	(54,88.32)	(55,88.19)	(56,88.45)	(57,88.52)	(58,88.22)	(59,88.47)	(60,88.36)	(61,88.45)	(62,88.62)	(63,88.42)	(64,88.48)	(65,88.41)	(66,88.51)	(67,88.56)	(68,88.69)	(69,88.44)	(70,88.55)	(71,88.58)	(72,88.49)	(73,88.51)	(74,88.38)	(75,88.52)	(76,88.63)	(77,88.68)	(78,88.59)	(79,88.49)	(80,88.44)	(81,88.33)	(82,88.63)	(83,88.65)	(84,88.89)	(85,88.41)	(86,88.5)	(87,88.6)	(88,88.61)	(89,88.49)	(90,88.67)	(91,88.85)	(92,88.62)	(93,88.74)	(94,88.54)	(95,88.74)	(96,88.9)	(97,88.67)	(98,88.62)	(99,88.47)	(100,88.85)
    };
\addplot[color=blue,]
    coordinates {
    (1,79.08)	(2,82.55)	(3,84.45)	(4,85.24)	(5,85.38)	(6,86.03)	(7,86.34)	(8,86.81)	(9,86.81)	(10,87.04)	(11,87.13)	(12,87.27)	(13,87.51)	(14,87.61)	(15,87.75)	(16,87.82)	(17,87.91)	(18,87.97)	(19,87.88)	(20,88.1)	(21,88.13)	(22,88.14)	(23,88.16)	(24,88.41)	(25,88.31)	(26,88.28)	(27,88.41)	(28,88.46)	(29,88.44)	(30,88.53)	(31,88.51)	(32,88.72)	(33,88.62)	(34,88.64)	(35,88.73)	(36,88.5)	(37,88.75)	(38,88.7)	(39,88.87)	(40,88.71)	(41,88.75)	(42,88.76)	(43,88.65)	(44,88.97)	(45,88.95)	(46,88.75)	(47,88.9)	(48,88.79)	(49,88.86)	(50,89)	(51,88.96)	(52,88.92)	(53,88.91)	(54,88.99)	(55,89.09)	(56,89.05)	(57,89.01)	(58,89.09)	(59,88.94)	(60,89.01)	(61,89.02)	(62,89.15)	(63,88.9)	(64,89.18)	(65,89.24)	(66,89.15)	(67,89.19)	(68,89.21)	(69,89.19)	(70,89.24)	(71,89.28)	(72,89.05)	(73,89.07)	(74,89.16)	(75,89.05)	(76,89.26)	(77,89.33)	(78,89.21)	(79,89.28)	(80,89.33)	(81,89.31)	(82,89.36)	(83,89.37)	(84,89.36)	(85,89.39)	(86,89.3)	(87,89.28)	(88,89.2)	(89,89.26)	(90,89.41)	(91,89.18)	(92,89.4)	(93,89.25)	(94,89.23)	(95,89.45)	(96,89.41)	(97,89.42)	(98,89.47)	(99,89.5)	(100,89.47)
    };
\addplot[color=green,]
    coordinates {
    (1,78.1)	(2,81.25)	(3,83.27)	(4,83.92)	(5,84.34)	(6,84.67)	(7,84.88)	(8,85.59)	(9,85.76)	(10,85.95)	(11,86.19)	(12,86.4)	(13,86.34)	(14,86.83)	(15,86.92)	(16,87.01)	(17,86.94)	(18,87.15)	(19,87.21)	(20,87.03)	(21,87.32)	(22,87.21)	(23,87.63)	(24,87.49)	(25,87.52)	(26,87.64)	(27,87.55)	(28,87.49)	(29,87.55)	(30,87.7)	(31,87.81)	(32,87.95)	(33,87.84)	(34,87.8)	(35,88.03)	(36,87.86)	(37,87.6)	(38,87.65)	(39,88.01)	(40,87.91)	(41,87.96)	(42,88.08)	(43,87.95)	(44,88.1)	(45,87.97)	(46,88.04)	(47,88.12)	(48,87.93)	(49,88.01)	(50,88.13)	(51,88.07)	(52,87.98)	(53,88.01)	(54,87.83)	(55,87.96)	(56,88.25)	(57,88.19)	(58,87.87)	(59,88.18)	(60,88.22)	(61,88.04)	(62,88.3)	(63,87.92)	(64,88.01)	(65,88.06)	(66,88.33)	(67,88.31)	(68,88.44)	(69,88.14)	(70,88.31)	(71,88.31)	(72,88.2)	(73,88.15)	(74,87.99)	(75,88.42)	(76,88.32)	(77,88.29)	(78,88.25)	(79,88.29)	(80,88.36)	(81,87.85)	(82,88.26)	(83,88.32)	(84,88.43)	(85,88.26)	(86,88.24)	(87,88.16)	(88,88.25)	(89,88.14)	(90,88.48)	(91,88.32)	(92,88.25)	(93,88.58)	(94,87.89)	(95,88.12)	(96,88.36)	(97,88.34)	(98,88.1)	(99,88.13)	(100,88.33)
    };
\addplot[color=pink,]
    coordinates {
    (1,77.69)	(2,81.65)	(3,83.87)	(4,84.75)	(5,85.13)	(6,85.56)	(7,85.78)	(8,86.42)	(9,86.68)	(10,86.52)	(11,87)	(12,87.07)	(13,87.09)	(14,87.48)	(15,87.33)	(16,87.58)	(17,87.5)	(18,87.61)	(19,87.71)	(20,87.74)	(21,88.01)	(22,87.98)	(23,88.02)	(24,88.29)	(25,88.11)	(26,88.2)	(27,88.3)	(28,88.23)	(29,88.19)	(30,88.29)	(31,88.32)	(32,88.5)	(33,88.6)	(34,88.59)	(35,88.5)	(36,88.63)	(37,88.49)	(38,88.45)	(39,88.71)	(40,88.5)	(41,88.52)	(42,88.61)	(43,88.45)	(44,88.9)	(45,88.71)	(46,88.62)	(47,88.73)	(48,88.77)	(49,88.78)	(50,88.93)	(51,88.79)	(52,88.78)	(53,88.72)	(54,88.85)	(55,88.92)	(56,88.88)	(57,88.81)	(58,88.86)	(59,88.93)	(60,88.9)	(61,88.87)	(62,88.95)	(63,88.82)	(64,88.9)	(65,88.99)	(66,89.06)	(67,88.84)	(68,89.09)	(69,89.15)	(70,88.98)	(71,89.07)	(72,88.67)	(73,89.06)	(74,88.9)	(75,88.77)	(76,89.06)	(77,88.99)	(78,88.9)	(79,88.95)	(80,89.16)	(81,88.99)	(82,89.07)	(83,89.26)	(84,89.22)	(85,89.01)	(86,88.9)	(87,89.15)	(88,88.93)	(89,89.21)	(90,89.14)	(91,89.19)	(92,89.11)	(93,89.18)	(94,88.91)	(95,89.35)	(96,89.25)	(97,89.27)	(98,89.24)	(99,89.38)	(100,89.44)
    };
\legend{No dropout, Standard $p=0.1$, SliceOut $p=0.1$, Standard $p=0.5$, SliceOut $p=0.5$}
\end{axis}
\end{tikzpicture}
